# Supplementary material for: Towards Robustness to Label Noise in Text Classification via Noise Modeling
Source: arXiv:2101.11214 source file (2021-11-07)
Supplement: Supplementary file 1 [file supp.tex]

\appendix
\noindent{\Large \textbf{Appendix}}

\section{Details of BMM}
We fit a 2-component Beta mixture model over the normalized training losses ($\mathcal{L}_{CE}(\hat{y}^{(c)},\cdot) \in [0,1]$) obtained after training the model for some warmup epochs $T_0$.
Similar to \citet{arazo19}, we observe that using a Beta mixture model works better than using a Gaussian mixture model as it allows for asymmetric distributions and can capture the short left-tails of the clean sample losses.
For a sample $(x,y)$ with normalized loss $\mathcal{L}_{CE}(\hat{y}^{(c)},y)=\ell$, the 2-component BMM can be represented as: 
\begin{align}
     &p(\ell) = \lambda_c \cdot p(\ell | \text{clean}) + \lambda_n \cdot p(\ell | \text{noisy}) \nonumber \\
     &p(\ell | \text{clean}) = \frac{\Gamma(\alpha_c + \beta_c)}{\Gamma(\alpha_c)\Gamma(\beta_c)}\ell^{\alpha_c-1}{(1-\ell)}^{\beta_c-1} \nonumber \\
     &p(\ell | \text{noisy}) = \frac{\Gamma(\alpha_n + \beta_n)}{\Gamma(\alpha_n)\Gamma(\beta_n)}\ell^{\alpha_n-1}{(1-\ell)}^{\beta_n-1} \nonumber 
\end{align}
where $\Gamma$ denotes the gamma distribution and $\alpha_{c/n}, \beta_{c/n}$ are the parameters corresponding to the individual clean/noisy BMMs. 
The mixture coefficients $\lambda_c$ and $\lambda_n$, and parameters ($\alpha_{c/n}, \beta_{c/n}$) are learnt using the EM algorithm. 
On fitting the BMM $\mathcal{B}$, for a given input $x$ with a normalized loss $\mathcal{L}_{CE}(\hat{y}^{(c)},y)=\ell$, we the posterior probability of $x$ having a clean label is given by:
\[
\mathcal{B}(x) = \frac{\lambda_c \cdot p(\ell | \text{clean})}{\lambda_c \cdot p(\ell | \text{clean}) + \lambda_n \cdot p(\ell | \text{noisy})}
\]

\section{Experimental Details}

\paragraph{Datasets}
We experiment with two popular datasets: (i) the TREC question-type classification dataset ~\cite{Li:2002:LQC:1072228.1072378}, and 
(ii) AG-News classification dataset ~\cite{10.1145/1062745.1062778}.
The statistics of the datasets are shown in Table~\ref{tab:datasets}.

\input{datasets_table}

\paragraph{Models}
We conduct experiments on two popular model architectures: word-LSTM~\cite{Hochreiter:1997:LSM:1246443.1246450} and word-CNN~\cite{kim2014convolutional}.
For word-LSTM, we use a 2-layer BiLSTM with hidden dimension of 150.
In the word-CNN, we use 300 kernel filters each of size 3, 4 and 5. 
We use the pre-trained GloVe  embeddings~\cite{pennington2014glove} for training both models.
We train models on TREC and AG-News for 100 and 30 epochs respectively.
We use an Adam optimizer with a learning rate of $10^{-5}$ and a dropout of $0.3$ during training.
For the noise model $N_M$, we use a simple 2-layer feedforward neural network, with the number of hidden units $n_{hidden}=4 {\cdot} n_{input}$.
We choose the inputs to the noise model $R_M(x)$ as per the class of label noise, as described in the main text. 
We conduct hyper-parameter tuning for the number of warmup epochs $T_0$ and $\beta$ using grid search over the ranges of \{6,10,20\} and \{2,4,6,8,10\} respectively.

\section{Full Results}
Tables \ref{tab:inp_trec} and \ref{tab:inp_ag} show the full results of our experiments on input-conditional noise. 
We report two metrics for each model trained: (i) \textit{Best}: the test accuracy of the model which achieves the best validation accuracy, and (ii) \textit{Last}: the test accuracy of the model obtained after the last training epoch.

\input{full_tables/results_inp_trec}

\vspace{-5em}

\input{full_tables/results_inp_ag}

\vspace{\fill}
